# Supplementary material for: Asymmetric Contextual Modulation for Infrared Small Target Detection
Source: arXiv:2009.14530 source file (2020-09-30)
Supplement: Supplementary file 1 [file appendix.tex]

% !TEX root = ../main.tex
%\bibliography{../reference}

{\Large{\textbf{Appendix}}}

\section{Accelerated Implementations}

Besides faithfully re-producing these state-of-the-arts models, for many non-learning based models, we also implement them with some accelerating schemes without harming the final performance. To elucidate how these schemes help, here are some examples:
\begin{enumerate}
  \item For the local contrast-based methods, given central and neighborhood feature maps, the local contrast map is generally calculated pixel-wisely \cite{TGRS13LCM,PR16MPCM}. However, it can be replaced with a cyclic shift on the whole feature maps to save time. For instance, with this exchanging trick, MPCM can be 15\% faster, increasing from 2.67 FPS to 3.07 FPS.
  \item For many low-rank based methods \cite{TIP13IPI}, the target-background separation is achieved via accelerated proximal gradient (APG) method \cite{FnT15ConvexOptim}, which is slow. To speed them up, for all low-rank based methods, we implement them with the Inexact Alternating Direction Method (IALM). 
  \item Again, for low-rank based methods, we add the stopping criteria proposed in \cite{JSTARS17RIPT} as a choice, which can save up to 50 times of the computational time.
\end{enumerate}

\section{Implementation details}
% \subsection{Implementation details}
We implemented all the learning-based methods in MXNet \cite{NIPSW15MXNet} and non-learning based methods in MATLAB.
For all learning-based methods, we choose to minimize the Soft-IoU loss function~\cite{SoftIoU} over the training set.
We adopt AdaGrad~\cite{COLT10Adagrad} as an optimizer with a learning rate of $0.1$ and the strategy described by He~\etal~\cite{He2015PReLU} for weight initialization, a total of 200 epochs, weight decay of $10^{-4}$, and a batch size of 10. 
To stack images of different sizes into a batch, each image is resized to $512 \times 512$ and randomly cropped to $480 \times 480$ during training.
The detailed hyper-parameter settings of the non-learning methods are listed in \cref{tab:params}.

\setlength{\tabcolsep}{4pt}
\begin{table*}[!h]
\caption{Detailed hyper-parameter settings of non-learning methods for comparison.}
\label{tab:params}
\centering
\small
\begin{tabular}{Sl Sl} 
\toprule
Methods & Hyper-parameter settings \\
\midrule
MPCM \cite{PR16MPCM} & $N=1,3,...,9$ \\
FKRW \cite{TGRS19FKRW} & $K=4$, $p=6$, $\beta=200$, window size:$ 11\times11$ \\
SMSL \cite{TGRS17SMSL} & Patch size: 50$\times$50, $\lambda = \frac{2\times L}{\sqrt{\min{(m,n)}}}$, $L=2.0$, threshold factor: $k=1$ \\
IPI \cite{TIP13IPI} & Patch size: 50$\times$50, stride: 10, $\lambda {\rm{ = }}L{\rm{/min(m,n}}{{\rm{)}}^{1/2}}$,$L=4.5$, threshold factor: $k=10$, $\varepsilon {\rm{ = 1}}{{\rm{0}}^{{\rm{ - 7}}}}$ \\
NIPPS \cite{IPT17NIPPS} &  Patch size: 50$\times$50, stride: 10, $\lambda = \frac{L}{\sqrt{\min{(m,n)}}}$, $L=2.0$, energy constraint ratio: $r=0.11$, threshold factor: $k=10$ \\
RIPT \cite{JSTARS17RIPT} &  Patch size: 50$\times$50, stride: 10, $\lambda = \frac{L}{\sqrt{\min{(I,J,P)}}}$, $L=0.001$, $h=0.1$, $\epsilon$=0.01, $\varepsilon = 10^{-7}$, threshold factor:$k=10$ \\
\bottomrule
\end{tabular}
\end{table*}
